# Supplementary material for: SyncTalk: The Devil is in the Synchronization for Talking Head Synthesis
Source: arXiv:2311.17590 source file (2024-04-28)
Supplement: Supplementary file 1 [file X_suppl.tex]

\clearpage
\setcounter{page}{1}
\maketitlesupplementary
